# Supplementary material for: A Field of Experts Prior for Adapting Neural Networks at Test Time
Source: arXiv:2202.05271 source file (2022-02-10)
Supplement: Supplementary file 1 [file appendix_old.tex]

% ===============================================
% ===============================================
\section{Appendix}

% =====================
% Approximating KL-divergence minimization of PoEs / FoEs with KL-divergence minimization of individual experts
% =====================
\subsection{Approximating KL-divergence minimization of PoEs / FoEs with KL-divergence minimization of individual experts}~\label{appendix_approximate_with_individual_KLs}
Consider PoE models for the source and target domain normalized images.
\begin{equation*}
    p^s(z) = \frac{\hat{p}^s(z)}{\mathcal{C}_s}, 
    \: \: \: \mathcal{C}_s = \int_z \hat{p}^s(z) dz,
    \: \: \: \hat{p}^s(z) = \prod_{j=1}^{J} p_j^s(u_j),
    \: \: \: u_j = f_j(z)
\end{equation*}
\begin{equation*}
    p^t(z) = \frac{\hat{p}^t(z)}{\mathcal{C}_t}, 
    \: \: \: \mathcal{C}_t = \int_z \hat{p}^t(z) dz,
    \: \: \: \hat{p}^t(z) = \prod_{j=1}^{J} p_j^t(u_j),
    \: \: \: u_j = f_j(z)
\end{equation*}

\noindent Here, we explicitly show the subscript $j$ in variables $u$ to indicate that different experts have different $1$D co-domains. Now, consider KL-divergence minimization between these distributions:
\begin{equation*}
    min_\phi \: D_{KL} (p^s(z), p^t(z)) \rightarrow min_\phi \: \int_z \: p^s(z) \: \log \: \frac{p^s(z)}{p^t(z)} \: dz
\end{equation*}
\begin{equation*}
    \rightarrow min_\phi \: \int_z \: \frac{\hat{p}^s(z)}{\mathcal{C}_s} \: \log \: \frac{\mathcal{C}_t}{\mathcal{C}_s} \: \frac{\hat{p}^s(z)}{\hat{p}^t(z)} \: dz
\end{equation*}
\begin{equation*}
    \rightarrow min_\phi \: \int_z \: \frac{\hat{p}^s(z)}{\mathcal{C}_s} \: \log \: \frac{\mathcal{C}_t}{\mathcal{C}_s} \: dz + \: \int_z \: \frac{\hat{p}^s(z)}{\mathcal{C}_s} \: \frac{\hat{p}^s(z)}{\hat{p}^t(z)} \: dz
\end{equation*}
% As $\mathcal{C}_s$ and $\mathcal{C}_t$ do not depend on $z$ (it is integrated out), we have:
% \begin{equation*}
%     = min_\phi \: \frac{1}{\mathcal{C}_s} \: \log \: \frac{\mathcal{C}_t}{\mathcal{C}_s} \int_z \: \hat{p}^s(z) \: dz + \: \int_z \: \frac{\hat{p}^s(z)}{\mathcal{C}_s} \: \frac{\hat{p}^s(z)}{\hat{p}^t(z)} \: dz
% \end{equation*}
\begin{equation*}
    \rightarrow min_\phi \: \log \: \frac{\mathcal{C}_t}{\mathcal{C}_s} + \: \int_z \: \frac{\hat{p}^s(z)}{\mathcal{C}_s} \: \frac{\hat{p}^s(z)}{\hat{p}^t(z)} \: dz
\end{equation*}

\noindent Note that during TTA, $\phi$ is fixed for computing the source-domain distribution, while is variable for computing the target-domain distribution.
Thus, ignoring the 'source-domain-only' terms, the minimization can be stated as follows:
\begin{equation*}
    \rightarrow min_\phi \: \log \: \mathcal{C}_t + \int_z \: \hat{p}^s(z) \: \log \: \frac{\hat{p}^s(z)}{\hat{p}^t(z)} \: dz
\end{equation*}
\begin{equation*}
    \rightarrow min_\phi \: \log \: \mathcal{C}_t + \int_{u_1,u_2,..u_J} \: \prod_{j=1}^{J} p_j^s(u_j) \: \log \: \frac{\prod_{j=1}^{J} p_j^s(u_j)}{\prod_{j=1}^{J} p_j^t(u_j)} \: du_1du_2...du_J
\end{equation*}
\begin{equation*}
    \rightarrow min_\phi \: \log \: \mathcal{C}_t + \sum_{j=1}^{J} \: \int_{u_1,u_2,..u_J} \: \prod_{j=1}^{J} p_j^s(u_j) \: \log \: \frac{p_j^s(u_j)}{p_j^t(u_j)} \: du_1du_2...du_J
\end{equation*}
\begin{equation*}
    \rightarrow min_\phi \: \log \: \mathcal{C}_t + \sum_{j=1}^{J} \: \int_{u_j} \: p_j^s(u_j) \: \log \: \frac{p_j^s(u_j)}{p_j^t(u_j)} \: du_j
\end{equation*}

\noindent As the normalization constant $\mathcal{C}_t$ is intractable, we ignore it in our optimization:
\begin{equation*}
    \approx min_\phi \: \sum_{j=1}^{J} \: \int_{u_j} \: p_j^s(u_j) \: \log \: \frac{p_j^s(u_j)}{p_j^t(u_j)} \: du_j
\end{equation*}
\begin{equation*}
    \rightarrow min_\phi \: \sum_{j=1}^{J} \: D_{KL}(p_j^s(u_j), p_j^t(u_j))
\end{equation*}


% =====================
% How to incorporate information from multiple training subjects?
% =====================
\subsection{How to incorporate information from multiple training subjects?}~\label{appendix_multiple_training_subjects}
Consider the KL-divergence between the expected distribution over all training subjects and the distribution of the test subject. For simplicity of notation, let us consider only one $1$D expert's distribution.
\begin{equation*}
    D_{KL}\big{(}E_{p(s)}[p^s(u)], p^t(u)\big{)}
\end{equation*}
\begin{equation*}
    = \int_u \Big{(} \int_s p(s) p^s(u) ds \Big{)} \: log \: \frac{\int_s p(s) p^s(u) ds}{p^t(u)} \: du
\end{equation*}
\begin{equation*}
    = \int_s p(s) \Big{(} \int_u p^s(u) \: log \: \frac{\int_s p(s) p^s(u) ds}{p^t(u)} \: du \Big{)} ds
\end{equation*}
\begin{equation*}
    = \int_s p(s) \Big{(} \int_u p^s(u) \: log \: \frac{\int_s p(s) p^s(u) ds}{p^t(u)} \: \frac{p^s(u)}{p^s(u)} \: du \Big{)} ds
\end{equation*}
\begin{equation*}
    = \int_s p(s) \Big{(} \int_u p^s(u) \: log \: \frac{\int_s p(s) p^s(u) ds}{p^s(u)} \: du + \: \int_u p^s(u) \: log \: \frac{p^s(u)}{p^t(u)} \: du \Big{)} ds
\end{equation*}
\begin{equation*}
    = \int_s p(s) \Big{(} \int_u p^s(u) \: log \: \frac{E_{p(s)}[p^s(u)]}{p^s(u)} \: du + \: \int_u p^s(u) \: log \: \frac{p^s(u)}{p^t(u)} \: du \Big{)} ds
\end{equation*}
\begin{equation*}
    = - \: \E_{p(s)}[D_{KL}(p^s(u), E_{p(s)}[p^s(u)])] + \E_{p(s)}[D_{KL}(p^s(u), p^t(u))]
\end{equation*}
\begin{equation*}
    \leq \E_{p(s)}[D_{KL}(p^s(u), p^t(u))]
\end{equation*}

% ================
% PCA related figures
% ================
\subsection{PCA related figures (prostate segmentation)}
\begin{figure}[h!]
\centering
    \includegraphics[trim = 0mm 120mm 0mm 0mm, angle=0, clip, width=0.7\textwidth]{figures/SD_features_c13.png}
\caption{Features of one channel in the last-but-one layer from central slices of different source domain training subjects.}~\label{fig_last_layer_features}
\end{figure}

\begin{figure}[h!]
\centering
    \includegraphics[trim = 0mm 120mm 0mm 0mm, angle=0, clip, width=0.7\textwidth]{figures/SD_patches_c13.png}
\caption{Examples of extracted patches from the features shown in Fig.~\ref{fig_last_layer_features}}~\label{fig_last_layer_patches}
\end{figure}

\begin{figure}[h!]
\centering
    \includegraphics[trim = 0mm 120mm 0mm 0mm, angle=0, clip, width=0.7\textwidth]{figures/SD_active_patches_c13.png}
\caption{Examples of 'Active' patches (those whose central pixel has a value greater that $\tau = 0.8$ in the predicted non-background probability).}~\label{fig_last_layer_patches_active}
\end{figure}

% =====================
% Extensions / Variants of He 2021 to get optimal performance on the MRI segmentation task for the datasets used in our experiments
% =====================
\newpage
\subsection{Extensions / Variants of He 2021 to get optimal performance on the MRI segmentation task for the datasets used in our experiments}~\label{appendix_he_2021_experiments}

We implement the test-time adaptation method proposed in ~\cite{he2021autoencoder}, within our network architecture. The base task network in our work is similar to theirs, with two differences: (a) we use two convolutional layers at each depth, while they use one convolutional layer at each depth, (b) we train the normalization module $N_\phi$ ($3$x$3$ kernels) during the source-domain training and later update it for each test image, while they insert a randomly initialized adaptor module $A^X$ ($1$x$1$ kernels).
Accordingly, our training procedure is shown in Fig.~\ref{fig_he_2021_training}.
Here, in addition to training the normalization module $N_\phi$ and the segmentation network $S_\theta$, we train 5 autoencoders: $AE_X$, $AE_Y$, $AE_{F_1}$, $AE_{F_2}$ and $AE_{F_3}$.
At test time, 4 adaptors are introduced: $A^X$, $A^{F_1}$, $A^{F_2}$ and $A^{F_3}$, as shown in Fig.~\ref{fig_he_2021_tta}. In the following sub-sections, we describe the modifications to the original method~\cite{he2021autoencoder}, that we did to obtain optimal test-time adaptation performance on the datasets used in this work.

\begin{figure}[h!]
\centering
    \includegraphics[trim = 0mm 0mm 0mm 0mm, angle=0, clip, width=0.8\textwidth]{figures/he_train_2.PNG}
\caption{Training procedure in He 2021}~\label{fig_he_2021_training}
\end{figure}

\begin{figure}[h!]
\centering
    \includegraphics[trim = 0mm 0mm 0mm 0mm, angle=0, clip, width=0.8\textwidth]{figures/he_test_2.PNG}
\caption{TTA procedure in He 2021}~\label{fig_he_2021_tta}
\end{figure}

\subsubsection{Architecture of adaptors}

% =====================
% =====================
% \subsection*{A.3. Subject-wise results}
% % =======================================
% % TABLE - Subject-wise results
% % =======================================
% \begin{table}[h!]
%     \small
%     \centering
%     \begin{tabular}{|c|c|c|c|c|c|}
%         \hline
%         \rowcolor{titlegray} 
%         Subject ID & Baseline & TTA-Gaussian & TTA-KDE & TTA-PCA-KDE & Benchmark\\
%         \hline
%         0059 & 0.81 & 0.81 & 0.81 & 0.80 &  \\
%         0075 & 0.84 & 0.84 & 0.84 & 0.83 &  \\
%         0060 & 0.82 & 0.81 & 0.78 & 0.84 &  \\
%         0076 & 0.68 & 0.36 & 0.68 & 0.70 &  \\
%         0082 & 0.87 & 0.87 & 0.86 & 0.88 &  \\
%         0073 & 0.85 & 0.85 & 0.85 & 0.81 &  \\
%         0080 & 0.72 & 0.66 & 0.73 & 0.72 &  \\
%         0071 & 0.65 & 0.56 & 0.65 & 0.72 &  \\
%         0063 & 0.73 & 0.73 & 0.72 & 0.70 &  \\
%         0074 & 0.69 & 0.69 & 0.66 & 0.60 &  \\
%         \hline
%     \end{tabular}
%     \caption{BMC Subject-wise results}~\label{tab:subjectwise_results_bmc}
% \end{table}

% \begin{table}[h!]
%     \small
%     \centering
%     \begin{tabular}{|c|c|c|c|c|c|}
%         \hline
%         \rowcolor{titlegray} 
%         Subject ID & Baseline & TTA-Gaussian & TTA-KDE & TTA-PCA-KDE & Benchmark\\
%         \hline
%         88800036 & 0.72 & 0.75 & 0.76 & 0.76 &  \\
%         88800049 & 0.87 & 0.87 & 0.88 & 0.88 &  \\
%         88800057 & 0.70 & 0.69 & 0.70 & 0.72 &  \\
%         88800035 & 0.80 & 0.82 & 0.81 & 0.82 &  \\
%         88800039 & 0.80 & 0.80 & 0.80 & 0.80 &  \\
%         88800046 & 0.72 & 0.78 & 0.86 & 0.85 &  \\
%         88800038 & 0.79 & 0.79 & 0.83 & 0.84 &  \\
%         88800021 & 0.91 & 0.91 & 0.92 & 0.91 &  \\
%         88800068 & 0.81 & 0.81 & 0.80 & 0.78 &  \\
%         88800053 & 0.46 & 0.46 & 0.35 & 0.55 &  \\
%         \hline
%     \end{tabular}
%     \caption{USZ Subject-wise results}~\label{tab:subjectwise_results_usz}
% \end{table}

% \begin{table}[h!]
%     \small
%     \centering
%     \begin{tabular}{|c|c|c|c|c|c|}
%         \hline
%         \rowcolor{titlegray} 
%         Subject ID & Baseline & TTA-Gaussian & TTA-KDE & TTA-PCA-KDE & Benchmark\\
%         \hline
%         35 & 0.82 & 0.83 & 0.82 & 0.81 &  \\
%         34 & 0.81 & 0.81 & 0.82 & 0.80 &  \\
%         37 & 0.71 & 0.71 & 0.71 & 0.71 &  \\
%         36 & 0.86 & 0.86 & 0.85 & 0.85 &  \\
%         33 & 0.80 & 0.80 & 0.81 & 0.81 &  \\
%         32 & 0.70 & 0.64 & 0.65 & 0.68 &  \\
%         28 & 0.80 & 0.82 & 0.83 & 0.85 &  \\
%         29 & 0.68 & 0.82 & 0.83 & 0.85 &  \\
%         30 & 0.70 & 0.70 & 0.69 & 0.76 &  \\
%         31 & 0.85 & 0.88 & 0.88 & 0.91 &  \\
%         \hline
%     \end{tabular}
%     \caption{UCL Subject-wise results}~\label{tab:subjectwise_results_ucl}
% \end{table}

% \begin{table}[h!]
%     \small
%     \centering
%     \begin{tabular}{|c|c|c|c|c|c|}
%         \hline
%         \rowcolor{titlegray} 
%         Subject ID & Baseline & TTA-Gaussian & TTA-KDE & TTA-PCA-KDE & Benchmark\\
%         \hline
%         45 & 0.80 & 0.65 & 0.70 & 0.74 &  \\
%         48 & 0.85 & 0.80 & 0.84 & 0.82 &  \\
%         49 & 0.82 & 0.74 & 0.80 & 0.79 &  \\
%         46 & 0.68 & 0.80 & 0.83 & 0.85 &  \\
%         47 & 0.81 & 0.75 & 0.78 & 0.80 &  \\
%         41 & 0.81 & 0.72 & 0.81 & 0.79 &  \\
%         44 & 0.80 & 0.63 & 0.72 & 0.80 &  \\
%         43 & 0.85 & 0.85 & 0.84 & 0.88 &  \\
%         40 & 0.79 & 0.72 & 0.79 & 0.80 &  \\
%         42 & 0.92 & 0.92 & 0.92 & 0.91 &  \\
%         \hline
%     \end{tabular}
%     \caption{HK Subject-wise results}~\label{tab:subjectwise_results_hk}
% \end{table}

% \begin{table}[h!]
%     \small
%     \centering
%     \begin{tabular}{|c|c|c|c|c|c|}
%         \hline
%         \rowcolor{titlegray} 
%         Subject ID & Baseline & TTA-Gaussian & TTA-KDE & TTA-PCA-KDE & Benchmark\\
%         \hline
%         10 & 0.69 & 0.74 & 0.70 & 0.81 &  \\
%         12 & 0.66 & 0.82 & 0.66 & 0.82 &  \\
%         11 & 0.84 & 0.86 & 0.84 & 0.88 &  \\
%         08 & 0.76 & 0.79 & 0.76 & 0.78 &  \\
%         09 & 0.74 & 0.80 & 0.74 & 0.84 &  \\
%         03 & 0.41 & 0.70 & 0.76 & 0.77 &  \\
%         07 & 0.60 & 0.56 & 0.45 & 0.58 &  \\
%         05 & 0.55 & 0.74 & 0.70 & 0.78 &  \\
%         06 & 0.67 & 0.80 & 0.72 & 0.82 &  \\
%         04 & 0.40 & 0.33 & 0.54 & 0.75 &  \\
%         \hline
%     \end{tabular}
%     \caption{BIDMC Subject-wise results}~\label{tab:subjectwise_results_bidmc}
% \end{table}
